# Supplementary material for: InternImage: Exploring Large-Scale Vision Foundation Models with Deformable Convolutions
Source: arXiv:2211.05778 source file (2023-04-17)
Supplement: Supplementary file 1 [file supp_det_setting.tex]

\begin{tabular}{l|ccc|cc|c}
    
    \setlength\tabcolsep{0.97mm}
    settings & T & S & B & L & XL & H \\
    \hline
    Pre-training & \multicolumn{3}{c|}{IN-1K} & \multicolumn{2}{c|}{IN-22K} & O365 \\ 
    Detector & \multicolumn{3}{c|}{Mask R-CNN} & \multicolumn{2}{c|}{Cascade.} & DINO \\
    \hline
    Optimizer & \multicolumn{3}{c|}{AdamW} & \multicolumn{2}{c|}{AdamW} & AdamW \\
    LR & \multicolumn{3}{c|}{1e-4} & \multicolumn{2}{c|}{1e-4} & 1e-4 \\
    Layer-wise LR & \multicolumn{3}{c|}{1.0} & \multicolumn{2}{c|}{0.9} & 0.94 \\
    Train Epochs & \multicolumn{3}{c|}{36} & \multicolumn{2}{c|}{36} & 12 \\
    Drop Path    & 0.2 & 0.4 & 0.5 & 0.5 & 0.6 & 0.5 \\
    Batch Size & \multicolumn{3}{c|}{16} & \multicolumn{2}{c|}{16} & 64 \\
    Weight Decay & \multicolumn{3}{c|}{0.05} & \multicolumn{2}{c|}{0.05} & 0.0001 \\
    EMA & \multicolumn{3}{c|}{\no} & \multicolumn{2}{c|}{\no} & \no \\
    
\end{tabular}
