# Supplementary material for: InternImage: Exploring Large-Scale Vision Foundation Models with Deformable Convolutions
Source: arXiv:2211.05778 source file (2023-04-17)
Supplement: Supplementary file 2 [file supp_tensorrt.tex]

\begin{tabular}{l|c|c|c}
    \multirow{2}{*}{method} & \multicolumn{3}{|c|}{batch size} \\
     & 128 & 32 & 12\\
    \hline
    \model-T & 1.22 & 4.81 & 18.87 \\
    \model-S & 1.70 & 6.76 & 26.32 \\
    \model-B & 2.39 & 9.43 & 37.04 \\
\end{tabular}
