# Supplementary material for: InternImage: Exploring Large-Scale Vision Foundation Models with Deformable Convolutions
Source: arXiv:2211.05778 source file (2023-04-17)
Supplement: Supplementary file 3 [file supp_tiny_setting.tex]

\begin{tabular}{c|c}
    
    \setlength\tabcolsep{0.97mm}
    configuration & value \\
    \hline
    optimizer & AdamW \\
    base learning rate & 5e-4 \\
    warmup learning rate & 5e-7 \\
    learning rate schedule & cosine decay \\
    train epochs & 300 \\
    warmup epochs & 20 \\
    batch size & 4096 \\
    weight decay & 0.05 \\
    EMA decay & 0.9999 \\
    input size  & $224\times224$ \\
    kernel size & $3\times3$ \\
    normalization type & LN \\
    MLP ratio & 4.0 \\
    drop path rate & 0.1 \\
    mix up & 0.8 \\
    cut mix & 1.0 \\
    color jitter & 0.4 \\
\end{tabular}
